# Supplementary material for: Cross-dimensional valley excitons from F\"{o}rster coupling in arbitrarily twisted stacks of monolayer semiconductors
Source: arXiv:2212.02449 source file (2022-12-05)
Supplement: Supplementary file 1 [file Supp.pdf]

# Supplementary: Cross-dimensional valley excitons from Förster coupling in arbitrarily twisted stacks of monolayer semiconductors

Ci Li[1,2] and Wang Yao[1,2,*]

[1]*Department of Physics, The University of Hong Kong, Hong Kong, China*

[2]*HKU-UCAS Joint Institute of Theoretical and Computational Physics at Hong Kong, China*

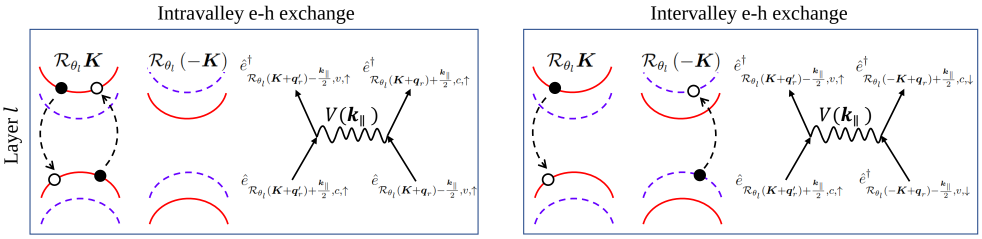


FIG. S1. (Color online) The intra- or intervalley electron-hole (e-h) exchange interaction (intralayer e-h exchange) depicted in terms of the conduction and valance states of electrons in the layer $l$ with the twist angle $\theta_l$, $\mathcal{R}_{\theta_l}$ is the rotational operator in the momentum space. The conduction-band electron in $\mathcal{R}_{\theta_l}K$ valley is scattered to the valance state in the same valley, while the valance-band electron in $\mathcal{R}_{\theta_l}K/\mathcal{R}_{\theta_l}(-K)$ valley is scattered to the conduction state in valley $\mathcal{R}_{\theta_l}K/\mathcal{R}_{\theta_l}(-K)$, as indicated by the dashed black arrows. The relative wave vector (to the valley $\mathcal{R}_{\theta_l}K$ or $\mathcal{R}_{\theta_l}K(-K)$) $\boldsymbol{q}_r$, $\boldsymbol{q}_r^{'}$, and in-plane center-of-mass momentum $\boldsymbol{k}_{\parallel}$ have been denoted in the plot.

## ELECTRON-HOLE EXCHANGE BETWEEN INTRALAYER EXCITONS IN DIFFERENT TRANSITION METAL DICHALCOGENIDE LAYERS

The exchange interaction between intralayer excitons in two different transition metal dichalcogenide (TMD) layers (such as the $l$ and $l'$ layers we assumed in the main text) is known as the Förster coupling [1–4]. It is induced by the Coulomb interaction between two nanostructures with a relatively long distance [2–4]. The Förster coupling has a similar form to the electron-hole (e-h) exchange between intralayer excitons of the same or different valleys in the monolayer TMD [5, 6], adding an exponential factor depending on the absolute value of in-plane centre-of-mass (COM) momentum $\boldsymbol{k}_{\parallel} = \left(k_{\parallel}\cos\varphi, k_{\parallel}\sin\varphi\right)$ and vertical distance between two layers $\Delta z$ [2–4].

### e-h exchange between intralayer excitons of same or different valleys in the same TMD layer

This kind of exchange has been well studied previously [5–7]. One can get the approximate expressions by straightly calculating the Coulomb exchange interaction between excitons in the same or different valleys [5, 6], or solving the Bethe-Salpeter equation (BSE) for e-h pair excitations [7]. Our derivation is based on the first ap-

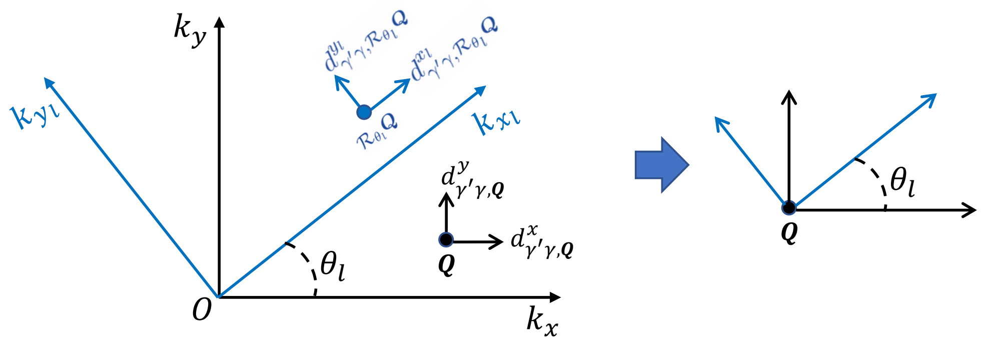


FIG. S2. (Color online) The schematic illustration of the relation between the optical transition dipole $\boldsymbol{d}_{\gamma'\gamma,\boldsymbol{Q}}$ in the untwisted layer and twisted layer $l$. $\boldsymbol{Q}$ represents the momentum near the $K$ or $-K$ valley. $\gamma'\gamma = vc$ or $cv$ is the band index for conduction ($c$) and valence ($v$) bands.

proach. For a specific layer $l$, one can define the creation operator for a bright exciton with in-plane COM momentum $\boldsymbol{k}_\parallel = \left(k_\parallel \cos\varphi, k_\parallel \sin\varphi\right)$ and relative twisted angle $\theta_l$ (to the untwisted layer): $\hat{B}^\dagger_{\boldsymbol{k}_\parallel,K}(l) \equiv \sum_{\boldsymbol{q}_r} \psi\left(\mathcal{R}_{\theta_l}\boldsymbol{q}_r\right) \hat{e}^\dagger_{\mathcal{R}_{\theta_l}(\boldsymbol{K}+\boldsymbol{q}_r)+\boldsymbol{k}_\parallel/2,\uparrow} \hat{h}^\dagger_{\mathcal{R}_{\theta_l}(-\boldsymbol{K}-\boldsymbol{q}_r)+\boldsymbol{k}_\parallel/2,\Downarrow}$ $\left(\hat{B}^\dagger_{\boldsymbol{k}_\parallel,-K}(l) \equiv \sum_{\boldsymbol{q}_r} \psi\left(\mathcal{R}_{\theta_l}\boldsymbol{q}_r\right) \hat{e}_{\mathcal{R}_{\theta_l}(-\boldsymbol{K}+\boldsymbol{q}_r)+\boldsymbol{k}_\parallel/2,\downarrow} \hat{h}^\dagger_{\mathcal{R}_{\theta_l}(\boldsymbol{K}-\boldsymbol{q}_r)+\boldsymbol{k}_\parallel/2,\Uparrow}\right)$, $\mathcal{R}_{\theta_l}\boldsymbol{q}_r$ $\left[\psi\left(\mathcal{R}_{\theta_l}\boldsymbol{q}_r\right)\right]$ is the relative wave vector [the wave function for the relative motion] between the electron and hole. Due to the stack of monolayers of the same TMD compound we considered, the only difference between different layers is the twisted angle $\theta_l$. The $l$ index has been dropped in $\psi\left(\mathcal{R}_{\theta_l}\boldsymbol{q}_r\right)$ for simplicity since $\sum_{\boldsymbol{q}_r}\psi(\mathcal{R}_{\theta_l}\boldsymbol{q}_r) \approx \sum_{\boldsymbol{q}_r}\psi(\boldsymbol{q}_r)$. The hole operator in the valence band is defined as $\hat{h}^\dagger_{\boldsymbol{k}_\parallel,\Downarrow(\Uparrow)} \equiv \hat{e}^\dagger_{v,-\boldsymbol{k}_\parallel,\uparrow(\downarrow)}$, and the electron operator in the conduction band $\hat{e}^\dagger_{\boldsymbol{k}_\parallel,\uparrow(\downarrow)} \equiv \hat{e}^\dagger_{c,\boldsymbol{k}_\parallel,\uparrow(\downarrow)}$. $\uparrow,\downarrow$ is the spin index.

$$\mathcal{R}_{\theta_l} \equiv \begin{pmatrix} \cos\theta_l & -\sin\theta_l \\ \sin\theta_l & \cos\theta_l \end{pmatrix},$$

is a rotational operator in the momentum space, as shown in Fig. S1. $\mathcal{R}_{\theta_l}\boldsymbol{Q}$ means twisting the momentum $\boldsymbol{Q}$ for angle $\theta_l$ in the counterclockwise direction, which comes from the rotational operation $\mathcal{R}^{-1}_{\theta_l}\boldsymbol{r} = \mathcal{R}_{-\theta_l}\boldsymbol{r}$ in the real space. According to this definition, the basis of valley excitons that we used in the main text can be expressed as

$$\left|l,\boldsymbol{k}_\parallel\right\rangle_K \equiv \hat{B}^\dagger_{\boldsymbol{k}_\parallel,K}(l)\left|0\right\rangle, \left|l,\boldsymbol{k}_\parallel\right\rangle_{-K} \equiv \hat{B}^\dagger_{\boldsymbol{k}_\parallel,-K}(l)\left|0\right\rangle, \tag{1}$$

$|0\rangle$ is the vacuum state for intralayer excitons and

$$\begin{pmatrix} \left\langle l,\boldsymbol{k}_\parallel\right|_K \\ \left\langle l,\boldsymbol{k}_\parallel\right|_{-K} \end{pmatrix} H^l_{\text{intra}} \left(\left|l,\boldsymbol{k}_\parallel\right\rangle_K, \left|l,\boldsymbol{k}_\parallel\right\rangle_{-K}\right) \equiv \begin{pmatrix} J^l_{K,K} & J^l_{K,-K} \\ J^l_{-K,K} & J^l_{-K,-K} \end{pmatrix}, \tag{2}$$

as we mentioned in the main text. In detail [5, 6], the e-h intra- or intervalley exchange is

$$\begin{aligned}
J^{l}_{K,K} &= \sum_{\boldsymbol{q}_r \boldsymbol{q}'_r} \psi^{*}\left(\mathcal{R}_{\theta_l}\boldsymbol{q}_r\right)\psi\left(\mathcal{R}_{\theta_l}\boldsymbol{q}'_r\right) J^{l}_{K,K}\left(\mathcal{R}_{\theta_l}\boldsymbol{q}_r, \mathcal{R}_{\theta_l}\boldsymbol{q}'_r, \boldsymbol{k}_{\parallel}\right) \\
&= \sum_{\boldsymbol{G}} \frac{V\left(\boldsymbol{G}+\boldsymbol{k}_{\parallel}\right)}{A} \sum_{\boldsymbol{q}'_r}\left[\psi\left(\mathcal{R}_{\theta_l}\boldsymbol{q}'_r\right)\left\langle u_{\mathcal{R}_{\theta_l}(\boldsymbol{K}+\boldsymbol{q}'_r)+\boldsymbol{k}_{\parallel}/2,c,\uparrow}\right| e^{i\boldsymbol{G}\cdot\boldsymbol{r}}\left| u_{\mathcal{R}_{\theta_l}(\boldsymbol{K}+\boldsymbol{q}'_r)-\boldsymbol{k}_{\parallel}/2,v,\uparrow}\right\rangle\right] \\
&\quad\times \sum_{\boldsymbol{q}_r}\left[\psi^{*}\left(\mathcal{R}_{\theta_l}\boldsymbol{q}_r\right)\left\langle u_{\mathcal{R}_{\theta_l}(\boldsymbol{K}+\boldsymbol{q}_r)-\boldsymbol{k}_{\parallel}/2,v,\uparrow}\right| e^{-i\boldsymbol{G}\cdot\boldsymbol{r}}\left| u_{\mathcal{R}_{\theta_l}(\boldsymbol{K}+\boldsymbol{q}_r)+\boldsymbol{k}_{\parallel}/2,c,\uparrow}\right\rangle\right],
\end{aligned} \tag{3}$$

$$\begin{aligned}
J^{l}_{-K,-K} &= \sum_{\boldsymbol{G}} \frac{V\left(\boldsymbol{G}+\boldsymbol{k}_{\parallel}\right)}{A} \sum_{\boldsymbol{q}'_r}\left[\psi\left(\mathcal{R}_{\theta_l}\boldsymbol{q}'_r\right)\left\langle u_{\mathcal{R}_{\theta_l}(\boldsymbol{K}+\boldsymbol{q}'_r)+\boldsymbol{k}_{\parallel}/2,c,\downarrow}\right| e^{i\boldsymbol{G}\cdot\boldsymbol{r}}\left| u_{\mathcal{R}_{\theta_l}(\boldsymbol{K}+\boldsymbol{q}'_r)-\boldsymbol{k}_{\parallel}/2,v,\downarrow}\right\rangle\right] \\
&\quad\times \sum_{\boldsymbol{q}_r}\left[\psi^{*}\left(\mathcal{R}_{\theta_l}\boldsymbol{q}_r\right)\left\langle u_{\mathcal{R}_{\theta_l}(\boldsymbol{K}+\boldsymbol{q}_r)-\boldsymbol{k}_{\parallel}/2,v,\downarrow}\right| e^{-i\boldsymbol{G}\cdot\boldsymbol{r}}\left| u_{\mathcal{R}_{\theta_l}(\boldsymbol{K}+\boldsymbol{q}_r)+\boldsymbol{k}_{\parallel}/2,c,\downarrow}\right\rangle\right],
\end{aligned}$$

$$\begin{aligned}
J^{l}_{K,-K} &= \sum_{\boldsymbol{G}} \frac{V\left(\boldsymbol{G}+\boldsymbol{k}_{\parallel}\right)}{A} \sum_{\boldsymbol{q}'_r}\left[\psi\left(\mathcal{R}_{\theta_l}\boldsymbol{q}'_r\right)\left\langle u_{\mathcal{R}_{\theta_l}(\boldsymbol{K}+\boldsymbol{q}'_r)+\boldsymbol{k}_{\parallel}/2,c,\uparrow}\right| e^{i\boldsymbol{G}\cdot\boldsymbol{r}}\left| u_{\mathcal{R}_{\theta_l}(\boldsymbol{K}+\boldsymbol{q}'_r)-\boldsymbol{k}_{\parallel}/2,v,\uparrow}\right\rangle\right] \\
&\quad\times \sum_{\boldsymbol{q}_r}\left[\psi^{*}\left(\mathcal{R}_{\theta_l}\boldsymbol{q}_r\right)\left\langle u_{\mathcal{R}_{\theta_l}(\boldsymbol{K}+\boldsymbol{q}_r)-\boldsymbol{k}_{\parallel}/2,v,\downarrow}\right| e^{-i\boldsymbol{G}\cdot\boldsymbol{r}}\left| u_{\mathcal{R}_{\theta_l}(\boldsymbol{K}+\boldsymbol{q}_r)+\boldsymbol{k}_{\parallel}/2,c,\downarrow}\right\rangle\right] \\
&= \left(J^{l}_{-K,K}\right)^{*},
\end{aligned}$$

where $\boldsymbol{G}$ is the reciprocal lattice vector for the untwisted layer ($\theta_l = 0$), $A$ is the area of two-dimensional (2D) plane, $\phi_{\boldsymbol{Q},c/v,\uparrow/\downarrow}(\boldsymbol{r}) = e^{i\boldsymbol{Q}\cdot\boldsymbol{r}} u_{\boldsymbol{Q},c/v,\uparrow/\downarrow}(\boldsymbol{r})$ represents the Bloch wave function at the momentum $\boldsymbol{Q}$, and $V\left(\boldsymbol{k}_{\parallel}\right) = \int V(\boldsymbol{r})\, e^{i\boldsymbol{k}_{\parallel}\cdot\boldsymbol{r}} d\boldsymbol{r}$ denotes the Coulomb potential in $\boldsymbol{k}_{\parallel}$ space. These terms can be divided into two parts: the long range part with $\boldsymbol{G} = 0$, and the short range part with $\boldsymbol{G} \neq 0$. The long range part has the form

$$\begin{aligned}
J^{l}_{\pm K,\pm K}(\boldsymbol{G}=0) &= \frac{V\left(\boldsymbol{k}_{\parallel}\right)}{A} \sum_{\boldsymbol{q}'_r} \psi\left(\mathcal{R}_{\theta_l}\boldsymbol{q}'_r\right)\left\langle u_{\mathcal{R}_{\theta_l}(\pm\boldsymbol{K}+\boldsymbol{q}'_r)+\boldsymbol{k}_{\parallel}/2,c}\right.\left| u_{\mathcal{R}_{\theta_l}(\pm\boldsymbol{K}+\boldsymbol{q}'_r)-\boldsymbol{k}_{\parallel}/2,v}\right\rangle \\
&\quad\times \sum_{\boldsymbol{q}_r} \psi^{*}\left(\mathcal{R}_{\theta_l}\boldsymbol{q}_r\right)\left\langle u_{\mathcal{R}_{\theta_l}(\pm\boldsymbol{K}+\boldsymbol{q}_r)-\boldsymbol{k}_{\parallel}/2,v}\right.\left| u_{\mathcal{R}_{\theta_l}(\boldsymbol{K}+\boldsymbol{q}_r)+\boldsymbol{k}_{\parallel}/2,c}\right\rangle.
\end{aligned} \tag{4}$$

where we have omitted the spin index for simplicity. Using the $\boldsymbol{k}\cdot\boldsymbol{p}$ expansion to expand $\left| u_{\mathcal{R}_{\theta_l}(\pm\boldsymbol{K}+\boldsymbol{q}_r)\pm\boldsymbol{k}_{\parallel}/2,c/v}\right\rangle$ in the first order of $k_{\parallel}$, it gives

$$\begin{aligned}
&\left| u_{\mathcal{R}_{\theta_l}(\pm\boldsymbol{K}+\boldsymbol{q}_r)\pm\boldsymbol{k}_{\parallel}/2,c/v}\right\rangle \\
&= \left| u_{\mathcal{R}_{\theta_l}(\pm\boldsymbol{K}+\boldsymbol{q}_r),c/v}\right\rangle \mp \frac{\boldsymbol{k}_{\parallel}}{2}\cdot\sum_{\gamma'\neq\gamma} \boldsymbol{d}_{\gamma'\gamma,\mathcal{R}_{\theta_l}(\pm\boldsymbol{K}+\boldsymbol{q}_r)}\left| u_{\gamma',\mathcal{R}_{\theta_l}(\pm\boldsymbol{K}+\boldsymbol{q}_r)}\right\rangle + O\left(k_{\parallel}^{2}\right)
\end{aligned} \tag{5}$$

with $\boldsymbol{d}_{\gamma'\gamma,\boldsymbol{Q}} = \frac{\hbar}{m_e}\frac{\langle u_{\gamma',\boldsymbol{Q}}|\boldsymbol{p}|u_{\gamma,\boldsymbol{Q}}\rangle}{\varepsilon_{\gamma'}-\varepsilon_{\gamma}}, \boldsymbol{p} = -i\hbar\nabla, \gamma'\gamma = cv$ or $vc$ is the optical transition dipole between conduction ($c$) band and valence ($v$) band in the effective single-particle two-band $\boldsymbol{k}\cdot\boldsymbol{p}$ model near the valley, $m_e$ is the free electron mass, and $\varepsilon_{\gamma=c,v}$ corresponds to the dispersion of $c$ or $v$ band respectively. As we showed in Fig. S2, the relation between the optical transition dipole in the untwisted layer, and twisted layer $l$ with the twisted angle $\theta_l$ can be expressed as

$$d^{x_l}_{\gamma'\gamma,\mathcal{R}_{\theta_l}\boldsymbol{Q}} = d^{x}_{\gamma'\gamma,\boldsymbol{Q}},\, d^{y_l}_{\gamma'\gamma,\mathcal{R}_{\theta_l}\boldsymbol{Q}} = d^{y}_{\gamma'\gamma,\boldsymbol{Q}}.$$

So

$$\boldsymbol{d}_{\gamma'\gamma,\mathcal{R}_{\theta_l}(\pm\boldsymbol{K}+\boldsymbol{q}_r)} = \mathcal{R}_{\theta_l}\boldsymbol{d}_{\gamma'\gamma,\pm\boldsymbol{K}+\boldsymbol{q}_r}, \tag{6}$$

in the original untwisted Cartesian coordinate, which gives

$$\begin{aligned}
&\frac{\boldsymbol{k}_\parallel}{2}\cdot\sum_{\gamma'\neq\gamma}\boldsymbol{d}_{\gamma'\gamma,\mathcal{R}_{\theta_l}(\pm\boldsymbol{K}+\boldsymbol{q}_r)} = \frac{\boldsymbol{k}_\parallel}{2}\cdot\sum_{\gamma'\neq\gamma}\mathcal{R}_{\theta_l}\boldsymbol{d}_{\gamma'\gamma,\pm\boldsymbol{K}+\boldsymbol{q}_r} \qquad (7)\\
&=\frac{\boldsymbol{k}_\parallel}{2}\cdot\sum_{\gamma'\neq\gamma}\left(d^x_{\gamma'\gamma,\pm\boldsymbol{K}+\boldsymbol{q}_r}\cos\theta_l - d^y_{\gamma'\gamma,\pm\boldsymbol{K}+\boldsymbol{q}_r}\sin\theta_l,\, d^x_{\gamma'\gamma,\pm\boldsymbol{K}+\boldsymbol{q}_r}\sin\theta_l + d^y_{\gamma'\gamma,\pm\boldsymbol{K}+\boldsymbol{q}_r}\cos\theta_l\right)^T\\
&=\sum_{\gamma'\neq\gamma}\{\frac{k_+}{4}\left[d^x_{\gamma'\gamma,\pm\boldsymbol{K}+\boldsymbol{q}_r}\cos\theta_l - d^y_{\gamma'\gamma,\pm\boldsymbol{K}+\boldsymbol{q}_r}\sin\theta_l - i\left(d^x_{\gamma'\gamma,\pm\boldsymbol{K}+\boldsymbol{q}_r}\sin\theta_l + d^y_{\gamma'\gamma,\pm\boldsymbol{K}+\boldsymbol{q}_r}\cos\theta_l\right)\right]\\
&\quad+\frac{k_-}{4}\left[d^x_{\gamma'\gamma,\pm\boldsymbol{K}+\boldsymbol{q}_r}\cos\theta_l - d^y_{\gamma'\gamma,\pm\boldsymbol{K}+\boldsymbol{q}_r}\sin\theta_l + i\left(d^x_{\gamma'\gamma,\pm\boldsymbol{K}+\boldsymbol{q}_r}\sin\theta_l + d^y_{\gamma'\gamma,\pm\boldsymbol{K}+\boldsymbol{q}_r}\cos\theta_l\right)\right]\\
&=\frac{k_+}{4}\sum_{\gamma'\neq\gamma}e^{-i\theta_l}d^-_{\gamma'\gamma,\pm\boldsymbol{K}+\boldsymbol{q}_r} + \frac{k_-}{4}\sum_{n'\neq c/v}e^{i\theta_l}d^+_{\gamma'\gamma,\pm\boldsymbol{K}+\boldsymbol{q}_r},
\end{aligned}$$

with $k_\pm = k_x \pm ik_y$, $d^\pm_{\gamma'\gamma,\pm\boldsymbol{K}+\boldsymbol{q}_r} = d^x_{\gamma'\gamma,\pm\boldsymbol{K}+\boldsymbol{q}_r} \pm id^y_{\gamma'\gamma,\pm\boldsymbol{K}+\boldsymbol{q}_r}$. Then

$$\begin{aligned}
\left\langle u_{\mathcal{R}_{\theta_l}(\pm\boldsymbol{K}+\boldsymbol{q}_r)-\boldsymbol{k}_\parallel/2,v}\right.\left|u_{\mathcal{R}_{\theta_l}(\pm\boldsymbol{K}+\boldsymbol{q}_r)+\boldsymbol{k}_\parallel/2,c}\right\rangle &\approx -\left(\frac{k_+}{4}e^{-i\theta_l}d^-_{vc,\pm\boldsymbol{K}+\boldsymbol{q}_r} + \frac{k_-}{4}e^{i\theta_l}d^+_{vc,\pm\boldsymbol{K}+\boldsymbol{q}_r}\right) \qquad (8)\\
&\quad+\left(\frac{k_+}{4}e^{-i\theta_l}d^-_{cv,\pm\boldsymbol{K}+\boldsymbol{q}_r} + \frac{k_-}{4}e^{i\theta_l}d^+_{cv,\pm\boldsymbol{K}+\boldsymbol{q}_r}\right)^*\\
&=\frac{1}{2}\left(k_+e^{-i\theta_l}d^-_{cv,\pm\boldsymbol{K}+\boldsymbol{q}_r} + k_-e^{i\theta_l}d^+_{cv,\pm\boldsymbol{K}+\boldsymbol{q}_r}\right)^*,\\
\left\langle u_{\mathcal{R}_{\theta_l}(\pm\boldsymbol{K}+\boldsymbol{q}'_r)+\boldsymbol{k}_\parallel/2,c,}\right.\left|u_{\mathcal{R}_{\theta_l}(\pm\boldsymbol{K}+\boldsymbol{q}'_r)-\boldsymbol{k}_\parallel/2,v}\right\rangle &\approx \left(\frac{k_+}{4}e^{-i\theta_l}d^-_{cv,\pm\boldsymbol{K}+\boldsymbol{q}'_r} + \frac{k_-}{4}e^{i\theta_l}d^+_{cv,\pm\boldsymbol{K}+\boldsymbol{q}'_r}\right)\\
&\quad-\left(\frac{k_+}{4}e^{-i\theta_l}d^-_{vc,\pm\boldsymbol{K}+\boldsymbol{q}'_r} + \frac{k_-}{4}e^{i\theta_l}d^+_{vc,\pm\boldsymbol{K}+\boldsymbol{q}'_r}\right)^*\\
&=\frac{1}{2}\left(k_+e^{-i\theta_l}d^-_{cv,\pm\boldsymbol{K}+\boldsymbol{q}'_r} + k_-e^{i\theta_l}d^+_{cv,\pm\boldsymbol{K}+\boldsymbol{q}'_r}\right),
\end{aligned}$$

leading to

$$\begin{aligned}
J^l_{\pm K,\pm K}\left(\boldsymbol{G}=0\right) &\approx \frac{V\left(\boldsymbol{k}_\parallel\right)}{A}\sum_{\boldsymbol{q}'_r}\psi\left(\mathcal{R}_{\theta_l}\boldsymbol{q}'_r\right)\frac{k_+e^{-i\theta_l}d^-_{cv,\pm\boldsymbol{K}+\boldsymbol{q}'_r}+k_-e^{i\theta_l}d^+_{cv,\pm\boldsymbol{K}+\boldsymbol{q}'_r}}{2} \qquad (9)\\
&\sum_{\boldsymbol{q}_r}\psi^*\left(\mathcal{R}_{\theta_l}\boldsymbol{q}_r\right)\frac{\left(k_+e^{-i\theta_l}d^-_{cv,\pm\boldsymbol{K}+\boldsymbol{q}_r}+k_-e^{i\theta_l}d^+_{cv,\pm\boldsymbol{K}+\boldsymbol{q}_r}\right)^*}{2}\\
&\approx \frac{V\left(\boldsymbol{k}_\parallel\right)}{4}\left(k_+e^{-i\theta_l}d^-_{cv,\pm\boldsymbol{K}}+k_-e^{i\theta_l}d^+_{cv,\pm\boldsymbol{K}}\right)\times\\
&\left(k_+e^{-i\theta_l}d^-_{cv,\pm\boldsymbol{K}}+k_-e^{i\theta_l}d^+_{cv,\pm\boldsymbol{K}}\right)^*\frac{1}{A}\sum_{\boldsymbol{q}'_r\boldsymbol{q}_r}\psi\left(\mathcal{R}_{\theta_l}\boldsymbol{q}'_r\right)\psi^*\left(\mathcal{R}_{\theta_l}\boldsymbol{q}_r\right)\\
&= \left|\psi\left(\boldsymbol{r}_{eh}=0\right)\right|^2\frac{V\left(\boldsymbol{k}_\parallel\right)}{4}\left(k_+e^{-i\theta_l}d^-_{cv,\pm\boldsymbol{K}}+k_-e^{i\theta_l}d^+_{cv,\pm\boldsymbol{K}}\right)\times\\
&\left(k_+e^{-i\theta_l}d^-_{cv,\pm\boldsymbol{K}}+k_-e^{i\theta_l}d^+_{cv,\pm\boldsymbol{K}}\right)^*.
\end{aligned}$$

$\psi\left(\boldsymbol{r}_{eh}\right)=\frac{1}{\sqrt{A}}\sum_{\boldsymbol{q}_r}\psi\left(\mathcal{R}_{\theta_l}\boldsymbol{q}_r\right)e^{-i\mathcal{R}_{\theta_l}\boldsymbol{q}_r\cdot\boldsymbol{r}_{eh}}$ is the real space wavefunction for the relative motion between electron and hole, which comes from solving the Schrodinger equation of the hydrogen-like atom [8]. $\rho(0)\equiv\left|\psi\left(\boldsymbol{r}_{eh}=0\right)\right|^2$ can be seen as the probability for electron and hole to overlap in an exciton. In the second step of the equation above, we have assumed that the exciton wavefunctions in the TMD are close to the Wannier type, i.e., well limited in the momentum space to a small neighborhood of the $\boldsymbol{K}$ and $-\boldsymbol{K}$ points, so $d^\pm_{cv,\boldsymbol{K}+\boldsymbol{q}_r}\approx d^\pm_{cv,\boldsymbol{K}}$. Here we would like to point out that $J^l_{K,-K}$ is gauge-dependent since the relative phase factor between excitonic states in different valleys can appear in this term. For the short range part of these exchanges, i.e., $J^l_{\pm K,\pm K}\left(\boldsymbol{G}\neq 0\right)$, the similar expansion used before shows

$$\begin{aligned}
J^l_{\pm K,\pm K}\left(\boldsymbol{G}\neq 0\right) = &\sum_{\boldsymbol{G}\neq 0}\frac{V\left(\boldsymbol{G}+\boldsymbol{k}_\parallel\right)}{A}\sum_{\boldsymbol{q}'_r}\left[\psi\left(\mathcal{R}_{\theta_l}\boldsymbol{q}'_r\right)\left\langle u_{\mathcal{R}_{\theta_l}\left(\pm\boldsymbol{K}+\boldsymbol{q}'_r\right)+\boldsymbol{k}_\parallel/2,c}\right|e^{i\boldsymbol{G}\cdot\boldsymbol{r}}\left|u_{\mathcal{R}_{\theta_l}\left(\pm\boldsymbol{K}+\boldsymbol{q}'_r\right)-\boldsymbol{k}_\parallel/2,v}\right\rangle\right]\\
&\times\sum_{\boldsymbol{q}_r}\left[\psi^*\left(\mathcal{R}_{\theta_l}\boldsymbol{q}_r\right)\left\langle u_{\mathcal{R}_{\theta_l}\left(\pm\boldsymbol{K}+\boldsymbol{q}_r\right)-\boldsymbol{k}_\parallel/2,v}\right|e^{-i\boldsymbol{G}\cdot\boldsymbol{r}}\left|u_{\mathcal{R}_{\theta_l}\left(\pm\boldsymbol{K}+\boldsymbol{q}_r\right)+\boldsymbol{k}_\parallel/2,c}\right\rangle\right]. \qquad (10)
\end{aligned}$$

The Fourier transformation of the Coulomb interaction can be calculated by choosing the polar coordinate to make $\boldsymbol{k}_\parallel$ to be parallel with the polar axis

$$\begin{aligned}
V\left(\boldsymbol{k}_\parallel\right) &= \int V\left(\boldsymbol{r}\right)e^{i\boldsymbol{k}_\parallel\cdot\boldsymbol{r}}d^2\boldsymbol{r} \qquad (11)\\
&= \int\frac{e^2}{4\pi\epsilon_0\epsilon_r r}e^{i\boldsymbol{k}_\parallel\cdot\boldsymbol{r}}d^2\boldsymbol{r}=\frac{e^2}{\epsilon}\int_0^\infty dr\int_0^{2\pi}e^{ik_\parallel r\cos\varphi_{in}}d\varphi_{in},
\end{aligned}$$

where we use the convention $\epsilon \equiv 4\pi\epsilon_0\epsilon_r$ for simplicity and $\varphi_{in}$ means the polar angle or azimuth in the polar coordinate. Since

$$
\begin{aligned}
\int_0^{2\pi} d\varphi_{in} e^{it\cos\varphi_{in}} &= \left(\int_0^{\pi} + \int_{\pi}^{2\pi}\right) d\varphi_{in} e^{it\cos\varphi_{in}} = \left(-\int_{2\pi}^{\pi} + \int_{\pi}^{2\pi}\right) d\varphi_{in} e^{it\cos\varphi_{in}} \\
&= 2\int_{\pi}^{2\pi} d\varphi_{in} e^{it\cos\varphi_{in}} = 2\int_0^{\pi} d\varphi_{in} e^{-it\cos\varphi_{in}} \\
&= 2\pi\mathcal{I}_0\left(it\right) = 2\pi\mathcal{J}_0\left(t\right),
\end{aligned} \tag{12}
$$

$\mathcal{J}_0\left(t\right)$ and $\mathcal{I}_0\left(it\right)$ is the Bessel function of the first and second kind respectively [9]. This derives

$$
\frac{e^2}{\epsilon}\int_0^{\infty} dr \int_0^{2\pi} e^{ik_{\parallel} r\cos\theta} d\theta = \frac{2\pi e^2}{\epsilon k_{\parallel}}\int_0^{\infty}\mathcal{J}_0\left(t\right) dt = \frac{2\pi e^2}{\epsilon k_{\parallel}}, \tag{13}
$$

which is the unscreened form of Coulomb interaction. Since $k_{\parallel} \ll |\boldsymbol{G}|$ in our consideration, $V\left(\boldsymbol{G}+\boldsymbol{k}_{\parallel}\right) \ll V\left(\boldsymbol{k}_{\parallel}\right)$ is always satisfied, which gives

$$
\begin{aligned}
J^l_{\pm K,\pm K}\left(\boldsymbol{G}\neq 0\right) &\approx J^l_{\pm K,\pm K}\left(\boldsymbol{G}\neq 0, \boldsymbol{k}_{\parallel}=0\right) \\
&= \sum_{\boldsymbol{G}\neq 0}\frac{V\left(\boldsymbol{G}\right)}{A}\sum_{\boldsymbol{q}'_r}\left[\psi\left(\mathcal{R}_{\theta_l}\boldsymbol{q}'_r\right)\left\langle u_{\mathcal{R}_{\theta_l}(\pm\boldsymbol{K}+\boldsymbol{q}'_r),c}\right| e^{i\boldsymbol{G}\cdot\boldsymbol{r}}\left|u_{\mathcal{R}_{\theta_l}(\pm\boldsymbol{K}+\boldsymbol{q}'_r),v}\right\rangle\right] \\
&\quad\times\sum_{\boldsymbol{q}_r}\left[\psi^*\left(\mathcal{R}_{\theta_l}\boldsymbol{q}_r\right)\left\langle u_{\mathcal{R}_{\theta_l}(\pm\boldsymbol{K}+\boldsymbol{q}_r),v}\right| e^{-i\boldsymbol{G}\cdot\boldsymbol{r}}\left|u_{\mathcal{R}_{\theta_l}(\pm\boldsymbol{K}+\boldsymbol{q}_r),c}\right\rangle\right] \\
&\approx \sum_{\boldsymbol{G}\neq 0}\frac{V\left(\boldsymbol{G}\right)}{A}\sum_{\boldsymbol{q}'_r}\left[\psi\left(\mathcal{R}_{\theta_l}\boldsymbol{q}'_r\right)\left\langle u_{\pm\mathcal{R}_{\theta_l}\boldsymbol{K},c}\right| e^{i\boldsymbol{G}\cdot\boldsymbol{r}}\left|u_{\pm\mathcal{R}_{\theta_l}\boldsymbol{K},v}\right\rangle\right] \\
&\quad\times\sum_{\boldsymbol{q}_r}\left[\psi^*\left(\mathcal{R}_{\theta_l}\boldsymbol{q}_r\right)\left\langle u_{\pm\mathcal{R}_{\theta_l}\boldsymbol{K},v}\right| e^{-i\boldsymbol{G}\cdot\boldsymbol{r}}\left|u_{\pm\mathcal{R}_{\theta_l}\boldsymbol{K},c}\right\rangle\right] \\
&\approx \sum_{\boldsymbol{G}\neq 0}\frac{V\left(\boldsymbol{G}\right)}{A}\sum_{\boldsymbol{q}'_r}\left[\psi\left(\boldsymbol{q}'_r\right)\left\langle u_{\pm\boldsymbol{K},c}\right| e^{i\boldsymbol{G}\cdot\boldsymbol{r}}\left|u_{\pm\boldsymbol{K},v}\right\rangle\right] \\
&\quad\times\sum_{\boldsymbol{q}_r}\left[\psi^*\left(\boldsymbol{q}_r\right)\left\langle u_{\pm\boldsymbol{K},v}\right| e^{-i\boldsymbol{G}\cdot\boldsymbol{r}}\left|u_{\pm\boldsymbol{K},c}\right\rangle\right],
\end{aligned} \tag{14}
$$

where we use the Wannier type of exciton wavefunctions in the TMD for the second approximation and $\left|u_{\pm\mathcal{R}_{\theta_l}\boldsymbol{K},c/v}\right\rangle \sim \left|u_{\pm\boldsymbol{K},c/v}\right\rangle$ for the last step in the above equation. Previous studies have proved that $J^l_{K,-K(-K,K)}\left(\boldsymbol{G}\neq 0, \boldsymbol{k}_{\parallel}=0\right)$ is forced to zero due to the three fold rotational symmetry in the monolayer TMD [5], while $J^l_{K,K(-K,-K)}\left(\boldsymbol{G}\neq 0, \boldsymbol{k}_{\parallel}=0\right)$ contributes the diagonal term in $H^l_{\text{intra}}$ as a total energy shift [6], which is in the order of $5 \sim 6\,\text{meV}$ and can be negligible in our consideration.

For the monolayer TMD, we have $\rho(0) \equiv \left|\psi\left(\boldsymbol{r}_{eh}=0\right)\right|^2 \sim 1/a_B^2$ with the exciton Bohr radius $a_B \approx 1\,\text{nm}$ [5, 8, 10], and $\boldsymbol{d}_{cv,\pm\boldsymbol{K}} = \left(\pm at/\varepsilon, -iat/\varepsilon\right)$ according to the single-particle

two-band $\boldsymbol{k}\cdot\boldsymbol{p}$ Hamiltonian [11]. Here the lattice constant $a$ of monolayer TMDs, the hopping amplitude $t$, and the band gap $\varepsilon$ can all be fitted from the ab *initio* band structures. One can easily find that

$$\begin{aligned}\frac{\left(k_- e^{i\theta_l} d^+_{cv,\boldsymbol{K}}\right)^*}{2} &= \frac{k_+ e^{-i\theta_l} d^-_{vc,\boldsymbol{K}}}{2} = \frac{k_+ e^{-i\theta_l}\left(d^x_{vc,\boldsymbol{K}} - i d^y_{vc,\boldsymbol{K}}\right)}{2} \\ &= \frac{k_+ e^{-i\theta_l} 2 d^x_{vc,\boldsymbol{K}}}{2} = e^{-i\theta_l}\left(\boldsymbol{k}_\parallel \cdot \boldsymbol{d}_{vc,\boldsymbol{K}}\right),\end{aligned}$$

$$\begin{aligned}\frac{\left(k_+ e^{-i\theta_l} d^-_{cv,-\boldsymbol{K}}\right)^*}{2} &= \frac{k_- e^{i\theta_l} d^+_{vc,-\boldsymbol{K}}}{2} = \frac{k_- e^{i\theta_l}\left(d^x_{vc,-\boldsymbol{K}} + i d^y_{vc,-\boldsymbol{K}}\right)}{2} \\ &= \frac{k_- e^{i\theta_l} 2 d^x_{vc,-\boldsymbol{K}}}{2} = e^{i\theta_l}\left(\boldsymbol{k}_\parallel \cdot \boldsymbol{d}_{vc,-\boldsymbol{K}}\right), \\ d^-_{cv,\boldsymbol{K}} &= d^+_{cv,-\boldsymbol{K}} = 0,\end{aligned}$$

since $d^x_{vc,\boldsymbol{K}} = -i d^y_{vc,\boldsymbol{K}} = \left|d^x_{vc,\boldsymbol{K}}\right| = -d^x_{vc,-\boldsymbol{K}} = -i d^y_{vc,-\boldsymbol{K}}$ in the monolayer TMD, which change $J^l_{\pm K,\pm K}$ (Eq. (9)) into

$$\begin{aligned}J^l_{K,K} &\approx \left|\psi\left(\boldsymbol{r}_{eh}=0\right)\right|^2 \frac{V\left(\boldsymbol{k}_\parallel\right)}{4}\left|k_+ e^{-i\theta_l} d^-_{cv,\boldsymbol{K}} + k_- e^{i\theta_l} d^+_{cv,\boldsymbol{K}}\right|^2 \\ &= \rho(0) V\left(\boldsymbol{k}_\parallel\right)\left|k_- e^{i\theta_l} d^+_{cv,\boldsymbol{K}}\right|^2/4 = \rho(0) V\left(\boldsymbol{k}_\parallel\right)\left|\boldsymbol{k}_\parallel \cdot \boldsymbol{d}_{cv,\boldsymbol{K}}\right|^2 \\ &= J^l_{-K,-K}, \\ J^l_{K,-K} &\approx \left|\psi\left(\boldsymbol{r}_{eh}=0\right)\right|^2 \frac{V\left(\boldsymbol{k}_\parallel\right)}{4}\left(k_- e^{i\theta_l} d^+_{cv,\boldsymbol{K}}\right)\left(k_+ e^{-i\theta_l} d^-_{cv,-\boldsymbol{K}}\right)^* \\ &= \rho(0) V\left(\boldsymbol{k}_\parallel\right) e^{2i\theta_l}\left(\boldsymbol{k}_\parallel \cdot \boldsymbol{d}_{cv,\boldsymbol{K}}\right)\left(\boldsymbol{k}_\parallel \cdot \boldsymbol{d}_{cv,-\boldsymbol{K}}\right)^* \\ &= \left(J^l_{-K,K}\right)^*.\end{aligned} \tag{15}$$

Combining with the expression of $V\left(\boldsymbol{k}_\parallel\right)$ (Eq. (13)), we finally have

$$\begin{aligned}J_{K,K} &\approx \frac{1}{a_B^2}\frac{2\pi e^2}{\epsilon k_\parallel}\frac{a^2 t^2}{\varepsilon^2} k_\parallel^2 = 2\pi \frac{e^2}{\epsilon a_B}\frac{a}{a_B}(aK)\frac{t^2}{\varepsilon^2}\frac{k_\parallel}{K} \\ &= J\frac{k_\parallel}{K} = J_{-K,-K}, \\ J^l_{K,-K} &\approx \frac{e^{2i\theta_l}}{a_B^2}\frac{2\pi e^2}{\epsilon k_\parallel}\frac{a^2 t^2}{\varepsilon^2}\left(k_x - i k_y\right)^2 = -J e^{2i\theta_l}\frac{k_\parallel}{K}\left(\frac{k_x - i k_y}{k}\right)^2 \\ &= -J\frac{k_\parallel}{K} e^{2i(\theta_l - \varphi)} = \left(J^l_{-K,K}\right)^*, \varphi = \arctan\left(k_y/k_x\right).\end{aligned} \tag{16}$$

Here the layer index $l$ for $J^l_{K,K(-K,-K)}$ has been dropped since this coupling is independent of it, as we used in the main text. $K \equiv 4\pi/3a$ is the distance from the $K$ to $\Gamma$ point, which gives the size of the Brillouin zone. $E_b = e^2/\left(\epsilon a_B\right)$ is the exciton binding energy

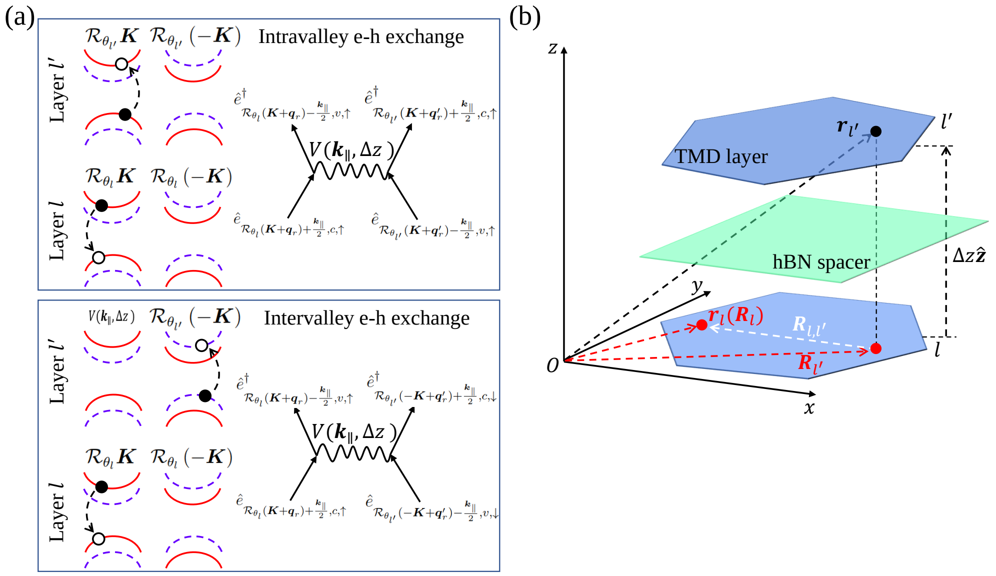


FIG. S3. (Color online)(a) Schematic illustration of the Förster coupling in the momentum space. Excitons in different TMD layers $l$ and $l'$ couple via the Förster mechanism under conservation of energy and momentum. (b) Illustration of the coordinate used for the Coulomb interaction in Eq. (20). Red and white (black) dashed arrows represent the in-plane (out-of-plane) vectors.

that equals $0.5 \sim 1\,\mathrm{eV}$ in monolayer TMDs [5, 8, 10, 12, 13]. By using the parameters of monolayer $WSe_2$: $a = 3.31\,\text{Å}$, $K = 1.26\,\text{Å}^{-1}$, $t = 1.19\,\mathrm{eV}$, $\varepsilon = 1.7\,\mathrm{eV}$ [5, 11], and considering $E_b = 0.5\,\mathrm{eV}$ in our calculation. It gives $J \approx 1\,\mathrm{eV}$ as used in the main text.

**e-h exchange between intralayer excitons of same or different valleys in different TMD layers**

Based on the derivation in the last subsection, we can calculate the e-h exchange interaction between any two layers ($l$ and $l'$), i.e., the Förster coupling, in a van der Waals stack from the same starting point. The Coulomb interaction used here is also dependent on the displacement in the $z$ direction, as shown in Fig. S3. Using the same basis we defined before, i.e, $\left\{\left|l,\boldsymbol{k}_\parallel\right\rangle_K, \left|l,\boldsymbol{k}_\parallel\right\rangle_K\right\}$, we have

$$\begin{pmatrix} \left\langle l,\boldsymbol{k}_\parallel\right|_K \\ \left\langle l,\boldsymbol{k}_\parallel\right|_{-K} \end{pmatrix} H_{\text{inter}}^{l,l'} \left(\left|l',\boldsymbol{k}_\parallel\right\rangle_K, \left|l',\boldsymbol{k}_\parallel\right\rangle_{-K}\right) \equiv \begin{pmatrix} J_{K,K}^{l,l'} & J_{K,-K}^{l,l'} \\ J_{-K,K}^{l,l'} & J_{-K,-K}^{l,l'} \end{pmatrix}. \tag{17}$$

In detail,

$$J^{l,l'}_{\pm K,\pm K} = \sum_{\boldsymbol{q}'_r \boldsymbol{q}'_r} \psi^* \left(\mathcal{R}_{\theta_{l'}} \boldsymbol{q}'_r\right) \psi \left(\mathcal{R}_{\theta_l} \boldsymbol{q}_r\right) J^{l,l'}_{\pm K,\pm K} \left(\mathcal{R}_{\theta_{l'}} \boldsymbol{q}'_r, \mathcal{R}_{\theta_l} \boldsymbol{q}_r, \boldsymbol{k}_\parallel\right), \tag{18}$$

with

$$\begin{aligned} & J^{l,l'}_{\pm K,\pm K} \left(\mathcal{R}_{\theta_{l'}} \boldsymbol{q}'_r, \mathcal{R}_{\theta_l} \boldsymbol{q}_r, \boldsymbol{k}_\parallel\right) \\ = & \int d\boldsymbol{r}_l d\boldsymbol{r}_{l'} \phi^*_{\mathcal{R}_{\theta_l}(\pm \boldsymbol{K}+\boldsymbol{q}_r)+\boldsymbol{k}_\parallel/2,c} \left(\boldsymbol{r}_l\right) \phi_{\mathcal{R}_{\theta_l}(\pm \boldsymbol{K}+\boldsymbol{q}_r)-\boldsymbol{k}_\parallel/2,v} \left(\boldsymbol{r}_l\right) V \left(\boldsymbol{r}_l - \boldsymbol{r}_{l'}\right) \\ & \times \phi_{\mathcal{R}_{\theta_{l'}}(\pm \boldsymbol{K}+\boldsymbol{q}'_r)+\boldsymbol{k}_\parallel/2,c} \left(\boldsymbol{r}_{l'}\right) \phi^*_{\mathcal{R}_{\theta_{l'}}(\pm \boldsymbol{K}+\boldsymbol{q}'_r)-\boldsymbol{k}_\parallel/2,v} \left(\boldsymbol{r}_{l'}\right), \end{aligned} \tag{19}$$

is the form of the Förster coupling in the momentum space [2–4], as shown in Fig. S3(a), where we have omitted the spin index for simplicity.

$$V \left(\boldsymbol{r}_l - \boldsymbol{r}_{l'}\right) = \frac{e^2}{\epsilon \left|\boldsymbol{r}_l - \boldsymbol{r}_{l'}\right|}, \tag{20}$$

also depends on the out-of-plane displacement, where vectors of real-space position can be written as $\boldsymbol{r}_l = \boldsymbol{R}_l$ and $\boldsymbol{r}_{l'} = \boldsymbol{R}_{l'} + \Delta z \hat{\boldsymbol{z}}$. $\boldsymbol{R}_{l'}$ is the projected in-plane vector of $\boldsymbol{r}_{l'}$ into $l$ layer. $\Delta z \equiv \left|\boldsymbol{z}_{l'} - \boldsymbol{z}_l\right|$ gives the distance between two layers in the $z$ direction, as shown in Fig. S3(b). Obviously, $\boldsymbol{r}_l - \boldsymbol{r}_{l'} = \boldsymbol{R}_l - \boldsymbol{R}_{l'} - \Delta z \hat{\boldsymbol{z}} = \boldsymbol{R}_{l,l'} - \Delta z \hat{\boldsymbol{z}}$ with $\boldsymbol{R}_{l,l'} \equiv \boldsymbol{R}_l - \boldsymbol{R}_{l'}$, so

$$\begin{aligned} V \left(\boldsymbol{r}_l - \boldsymbol{r}_{l'}\right) &= \frac{e^2}{\epsilon \left|\boldsymbol{r}_l - \boldsymbol{r}_{l'}\right|} = \frac{e^2}{\epsilon \left|\boldsymbol{R}_{l,l'} - \Delta z \hat{\boldsymbol{z}}\right|} \\ &= \sum_{\boldsymbol{G}} \frac{V \left(\boldsymbol{G} + \boldsymbol{k}_\parallel, \Delta z\right)}{A} e^{i\left(\boldsymbol{G}+\boldsymbol{k}_\parallel\right)\cdot \boldsymbol{R}_{l,l'}}, \end{aligned} \tag{21}$$

with

$$\begin{aligned} V \left(\boldsymbol{Q}, \Delta z\right) &= \int V \left(\boldsymbol{R}_{l,l'} - \Delta z \hat{\boldsymbol{z}}\right) e^{i\boldsymbol{Q}\cdot \boldsymbol{R}_{l,l'}} d^2 \boldsymbol{R}_{l,l'} \\ &= \int \frac{e^2}{\epsilon \left|\boldsymbol{R}_{l,l'} - \Delta z \hat{\boldsymbol{z}}\right|} e^{i\boldsymbol{Q}\cdot \boldsymbol{R}_{l,l'}} d^2 \boldsymbol{R}_{l,l'} \\ &= \frac{e^2}{\epsilon} \int_0^\infty R_{l,l'} dR_{l,l'} \int_0^{2\pi} \frac{e^{iQR_{l,l'}\cos\varphi_{in}}}{\sqrt{R^2_{l,l'} + \left(\Delta z\right)^2}} d\varphi_{in} \end{aligned} \tag{22}$$

is a Fourier transformation for the in-plane vector $\boldsymbol{R}_{l,l'}$. Using properties of the Bessel function shown in Eq. (12), it gives

$$\begin{aligned} & \frac{e^2}{\epsilon} \int_0^\infty R_{l,l'} dR_{l,l'} \int_0^{2\pi} \frac{e^{iQR_{l,l'}\cos\varphi_{in}}}{\sqrt{R^2_{l,l'} + \left(\Delta z\right)^2}} d\varphi_{in} \\ = & \frac{2\pi e^2}{\epsilon} \int_0^\infty \frac{R_{l,l'} \mathcal{J}_0 \left(QR_{l,l'}\right)}{\sqrt{R^2_{l,l'} + \left(\Delta z\right)^2}} dR_{l,l'} \\ = & \frac{2\pi e^2}{\epsilon Q} e^{-Q\Delta z}. \end{aligned} \tag{23}$$

Here the short-range part of $J^{l,l'}_{\pm K,\pm K}\left(\mathcal{R}_{\theta_{l'}}\boldsymbol{q}'_r,\mathcal{R}_{\theta_l}\boldsymbol{q}_r,\boldsymbol{k}_\parallel\right)$ still has the approximate form as

$$\begin{aligned}J^{l,l'}_{\pm K,\pm K}\left(\boldsymbol{G}\neq\boldsymbol{0},\boldsymbol{k}_\parallel\right)\approx J^{l,l'}_{\pm K,\pm K}\left(\boldsymbol{G}\neq 0,\boldsymbol{k}_\parallel=0\right)\\ \approx\sum_{\boldsymbol{G}\neq 0}\frac{V\left(\boldsymbol{G},\Delta z\right)}{A}\sum_{\boldsymbol{q}'_r}\left[\psi\left(\boldsymbol{q}_r\right)\left\langle u_{\pm\boldsymbol{K},c}\right|e^{i\boldsymbol{G}\cdot\boldsymbol{r}}\left|u_{\pm\boldsymbol{K},v}\right\rangle\right]\\ \times\sum_{\boldsymbol{q}_r}\left[\psi^*\left(\boldsymbol{q}'_r\right)\left\langle u_{\pm\boldsymbol{K},v}\right|e^{-i\boldsymbol{G}\cdot\boldsymbol{r}}\left|u_{\pm\boldsymbol{K},c}\right\rangle\right],\end{aligned}$$

since $V\left(\boldsymbol{G}+\boldsymbol{k}_\parallel,\Delta z\right)\ll V\left(\boldsymbol{k}_\parallel,\Delta z\right)$ is satisfied. Due to stack of monolayers of the same TMD compound we considered, the three fold rotational symmetry is still effective in the multilayer TMD system, leading to $J^{l,l'}_{K,-K(-K,K)}\left(\boldsymbol{G}\neq 0,\boldsymbol{k}_\parallel=0\right)=0$ as well as in the monolayer case. The diagonal part $J^{l,l'}_{K,K(-K,-K)}\left(\boldsymbol{G}\neq 0,\boldsymbol{k}_\parallel=0\right)$ is highly suppressed because of the exponential factor ($e^{-G\Delta z}\sim 10^{-10}$ for $\Delta z=1\,\mathrm{nm}$ and $a=3.31\,\mathrm{\AA}$), which can be ignored in our consideration. This means we only need to focus on the long-range limit (small $\boldsymbol{k}_\parallel$) for the Forster coupling, that is,

$$V\left(\boldsymbol{r}_l-\boldsymbol{r}_{l'}\right)\approx\frac{V\left(\boldsymbol{k}_\parallel,\Delta z\right)}{A}e^{i\boldsymbol{k}_\parallel\cdot\boldsymbol{R}_{l,l'}}. \tag{24}$$

Based on the Bloch wave functions $\phi_{\boldsymbol{Q},c/v,\uparrow/\downarrow}\left(\boldsymbol{r}_l\right)=e^{i\boldsymbol{Q}\cdot\boldsymbol{r}}u_{\boldsymbol{Q},c/v,\uparrow/\downarrow}\left(\boldsymbol{r}_l\right)$ at the momentum $\boldsymbol{Q}$, one can derive that

$$\begin{aligned}&J^{l,l'}_{\pm K,\pm K}\left(\mathcal{R}_{\theta_{l'}}\boldsymbol{q}'_r,\mathcal{R}_{\theta_l}\boldsymbol{q}_r,\boldsymbol{k}_\parallel\right)\\ &=\int d\boldsymbol{r}_l d\boldsymbol{r}_{l'}\phi^*_{\mathcal{R}_{\theta_l}(\pm\boldsymbol{K}+\boldsymbol{q}_r)+\boldsymbol{k}_\parallel/2,c}\left(\boldsymbol{r}_l\right)\phi_{\mathcal{R}_{\theta_l}(\pm\boldsymbol{K}+\boldsymbol{q}_r)-\boldsymbol{k}_\parallel/2,v}\left(\boldsymbol{r}_l\right)V\left(\boldsymbol{r}_l-\boldsymbol{r}_{l'}\right)\\ &\quad\times\phi_{\mathcal{R}_{\theta_{l'}}(\pm\boldsymbol{K}+\boldsymbol{q}'_r)+\boldsymbol{k}_\parallel/2,c}\left(\boldsymbol{r}_{l'}\right)\phi^*_{\mathcal{R}_{\theta_{l'}}(\pm\boldsymbol{K}+\boldsymbol{q}'_r)-\boldsymbol{k}_\parallel/2,v}\left(\boldsymbol{r}_{l'}\right)\\ &\approx\int d\boldsymbol{r}_l d\boldsymbol{r}_{l'}e^{-i\boldsymbol{k}_\parallel\cdot\boldsymbol{R}_l}u^*_{\mathcal{R}_{\theta_l}(\pm\boldsymbol{K}+\boldsymbol{q}_r)+\boldsymbol{k}_\parallel/2,c}\left(\boldsymbol{r}_l\right)u_{\mathcal{R}_{\theta_l}(\pm\boldsymbol{K}+\boldsymbol{q}_r)-\boldsymbol{k}_\parallel/2,v}\left(\boldsymbol{r}_l\right)\\ &\quad\times\frac{V\left(\boldsymbol{k}_\parallel,\Delta z\right)}{A}e^{i\boldsymbol{k}_\parallel\cdot\boldsymbol{R}_{l,l'}}\times\\ &\quad e^{i\boldsymbol{k}_\parallel\cdot\boldsymbol{R}_{l'}}u_{\mathcal{R}_{\theta_{l'}}(\pm\boldsymbol{K}+\boldsymbol{q}'_r)+\boldsymbol{k}_\parallel/2,c}\left(\boldsymbol{r}_{l'}\right)u^*_{\mathcal{R}_{\theta_{l'}}(\pm\boldsymbol{K}+\boldsymbol{q}'_r)-\boldsymbol{k}_\parallel/2,v}\left(\boldsymbol{r}_{l'}\right)\\ &=\frac{V\left(\boldsymbol{k}_\parallel,\Delta z\right)}{A}\left\langle u_{\mathcal{R}_{\theta_l}(\pm\boldsymbol{K}+\boldsymbol{q}_r)+\boldsymbol{k}_\parallel/2,c}\middle|\,u_{\mathcal{R}_{\theta_l}(\pm\boldsymbol{K}+\boldsymbol{q}_r)-\boldsymbol{k}_\parallel/2,v}\right\rangle\\ &\quad\times\left\langle u_{\mathcal{R}_{\theta_{l'}}(\pm\boldsymbol{K}+\boldsymbol{q}'_r)-\boldsymbol{k}_\parallel/2,v}\middle|\,u_{\mathcal{R}_{\theta_{l'}}(\pm\boldsymbol{K}+\boldsymbol{q}'_r)+\boldsymbol{k}_\parallel/2,c}\right\rangle.\end{aligned} \tag{25}$$

The last subsection has shown that

$$\begin{aligned}\left\langle u_{\mathcal{R}_{\theta_l}(\boldsymbol{K}+\boldsymbol{q}_r)+\boldsymbol{k}_\parallel/2,c}\middle|\,u_{\mathcal{R}_{\theta_l}(\boldsymbol{K}+\boldsymbol{q}_r)-\boldsymbol{k}_\parallel/2,v}\right\rangle&\approx e^{i\theta_l}\boldsymbol{k}_\parallel\cdot\boldsymbol{d}_{cv,\boldsymbol{K}},\\ \left\langle u_{\mathcal{R}_{\theta_{l'}}(\boldsymbol{K}+\boldsymbol{q}'_r)-\boldsymbol{k}_\parallel/2,v}\middle|\,u_{\mathcal{R}_{\theta_{l'}}(\boldsymbol{K}+\boldsymbol{q}'_r)+\boldsymbol{k}_\parallel/2,c}\right\rangle&\approx e^{-i\theta_{l'}}\boldsymbol{k}_\parallel\cdot\boldsymbol{d}_{vc,\boldsymbol{K}}\\ &=\left(e^{i\theta_{l'}}\boldsymbol{k}_\parallel\cdot\boldsymbol{d}_{cv,\boldsymbol{K}}\right)^*\end{aligned}$$

in monolayer TMDs, so

$$J_{K,K}^{l,l'}\left(\mathcal{R}_{\theta_{l'}}\boldsymbol{q}_r',\mathcal{R}_{\theta_l}\boldsymbol{q}_r,\boldsymbol{k}_\parallel\right)\approx\frac{2\pi e^2}{A\epsilon k_\parallel}e^{-k_\parallel\Delta z}e^{i(\theta_l-\theta_{l'})}\left|\boldsymbol{k}_\parallel\cdot\boldsymbol{d}_{cv,\boldsymbol{K}}\right|,$$

with

$$\begin{aligned}J_{K,K}^{l,l'}&=\sum_{\boldsymbol{q}_r\boldsymbol{q}_r'}\psi^*\left(\mathcal{R}_{\theta_{l'}}\boldsymbol{q}_r'\right)\psi\left(\mathcal{R}_{\theta_l}\boldsymbol{q}_r\right)J_{K,K}^{l,l'}\left(\mathcal{R}_{\theta_{l'}}\boldsymbol{q}_r',\mathcal{R}_{\theta_l}\boldsymbol{q}_r,\boldsymbol{k}_\parallel\right)\\&\approx\left|\psi\left(\boldsymbol{r}_{eh}=0\right)\right|^2\frac{2\pi e^2}{\epsilon k_\parallel}e^{-k_\parallel\Delta z}e^{i(\theta_l-\theta_{l'})}\left|\boldsymbol{k}_\parallel\cdot\boldsymbol{d}_{cv,\boldsymbol{K}}\right|\\&=J\frac{k_\parallel}{K}e^{-k_\parallel\Delta z}e^{i(\theta_l-\theta_{l'})}=\left(J_{-K,-K}^{l,l'}\right)^*.\end{aligned}\tag{26}$$

The similar process shows

$$J_{K,-K}^{l,l'}\approx-J\frac{k_\parallel}{K}e^{-k_\parallel\Delta z}e^{i(\theta_l+\theta_{l'})-2i\varphi}=\left(J_{-K,K}^{l,l'}\right)^*.\tag{27}$$

Here the form of the Coulomb interaction in the 2D momentum space, i.e.,

$$\frac{2\pi e^2}{\epsilon k_\parallel}e^{-k_\parallel\Delta z},$$

is a general consequence that the interlayer coupling induced by the Coulomb interaction has an exponential factor, which is dependent on the absolute value of in-plane momentum $\boldsymbol{k}_\parallel$ and vertical distance between two layers $\Delta z$. Previous studies have proved that the same from can be achieved from keeping only the dipole-dipole interaction after expanding the Coulomb interaction in Eq. (20) [2–4]. A similar form can also be obtained by taking the long-range limit (small $k_\parallel$) in the straightforward calculation of the interlayer interaction for the multilayer TMD heterostructure immersed in an anisotropic medium [16]

$$\begin{aligned}\mathcal{W}_{l,l'}\left(\boldsymbol{k}_\parallel\right)&=e^2\frac{2\pi e^{-k_\parallel\Delta z}}{\epsilon k_\parallel\left[\left(1+r_*^l k_\parallel\right)\left(1+r_*^{l'}k_\parallel\right)-r_*^l r_*^{l'}k_\parallel^2 e^{-2k_\parallel\Delta z}\right]}\\&\approx\frac{2\pi e^2}{\epsilon k_\parallel}e^{-k_\parallel\Delta z},\end{aligned}\tag{28}$$

which is solved from the Possion's equation with $r_*^{l(l')}$ is the corresponding monolayer screening lengths for layer $l$ ($l'$). Therefore, the standard form of Coulomb interaction we considered is a good approximation for the broadly-used Rytova-Keldysh form in TMD heterostructure calculations [14–16] when the momentum $\boldsymbol{k}_\parallel$ is enough small, where $\epsilon$ can be seen as an effective dielectric constant if the surrounding dielectric medium is anisotropic [16].

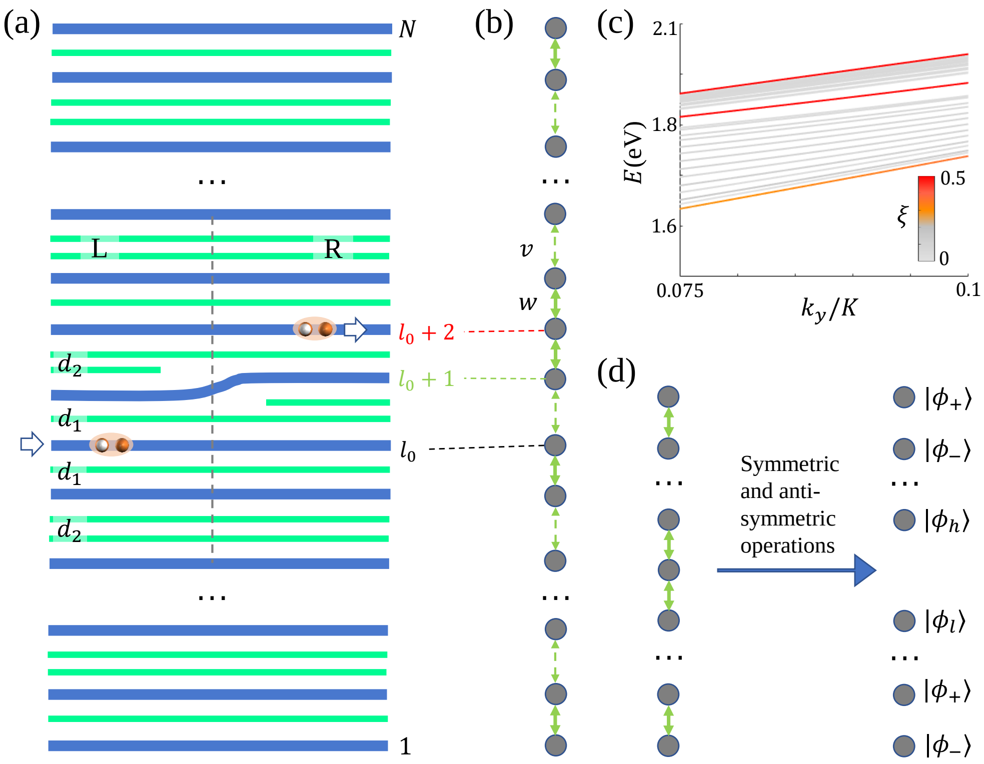


FIG. S4. (Color online) (a) Schematic of a TMD stack with an alternating thickness of spacers, mimicking the Su-Schrieffer-Heeger (SSH) chain. The interface part is the same as Fig. 4(a) in the main text. (b) An approximate coupled SSH chain corresponds to the R stack in (a) when $k_{\parallel}$ is large. (c) The zoom-in plot of Fig. 4(b) in the main text for $0.075 \le k_y/K \le 0.1$. (d) The effective chain when $w >> v$ and equivalent decoupled lattice structure after the symmetric and anti-symmetric operations.

At last, we replace the twist angle in the momentum space to the one in the real space, which leads to the form we used in the main text as

$$\begin{aligned}
J_{K,K} &\approx J\frac{k_{\parallel}}{K} = J_{-K,-K}, J^{l}_{K,-K} = -J\frac{k_{\parallel}}{K}e^{-2i(\theta_l+\varphi)} = \left(J^{l}_{-K,K}\right)^*, \\
J^{l,l'}_{K,K} &\approx J\frac{k_{\parallel}}{K}e^{-k_{\parallel}\Delta z}e^{-i(\theta_l-\theta_{l'})} = \left(J^{l,l'}_{-K,-K}\right)^*, \\
J^{l,l'}_{K,-K} &\approx -J\frac{k_{\parallel}}{K}e^{-k_{\parallel}\Delta z}e^{-i(\theta_l+\theta_{l'})-2i\varphi} = \left(J^{l,l'}_{-K,K}\right)^*.
\end{aligned} \tag{29}$$

## APPROXIMATE INTERFACE STATES IN THE COUPLED SSH CHAIN

According to the TMD stack shown in Fig. S4(a) (Fig. 4(a) in the main text), keeping only the nearest-neighbor Förster coupling justifiable at sufficiently large $k_{\parallel}$, the effective

SSH chain structure can be expressed as (Fig. S4(b))

$$H \simeq \sum_{s=1}^{(N+1-l_{\rm dw})/2} [w \left|l_{\rm dw}+2s-2\right\rangle_L \left\langle l_{\rm dw}+2s-1\right|_L + v \left|l_{\rm dw}+2s-1\right\rangle_L \left\langle l_{\rm dw}+2s\right|_L$$
$$+H.c.] + \sum_{s=1}^{l_{\rm dw}/2} [w \left|l_{\rm dw}-2s+2\right\rangle_L \left\langle l_{\rm dw}-2s+1\right|_L + v \left|l_{\rm dw}-2s+1\right\rangle_L \left\langle l_{\rm dw}-2s\right|_L$$
$$+H.c.] - v\left(\left|N\right\rangle_L \left\langle N+1\right|_L + \left|1\right\rangle_L \left\langle 0\right|_L + H.c.\right), \tag{30}$$

based on the basis of two branches having linearly polarized optical dipole longitudinal ($L$) and transverse ($T$) to exciton momentum respectively. $l_{\rm dw}$ represents the interface layer (domain wall) ($l_{\rm dw} = l_0$ for L stack and $l_0 + 2$ for R stack) as shown in Fig. S4(a). The global on-site energy $\varepsilon_L = \frac{\hbar^2 k_\parallel^2}{2m_X} + 2J\frac{k_\parallel}{K}$ has been omitted for simplicity, as well as the $\boldsymbol{k}_\parallel$ dependence in the basis. $N$ is the total layer number and

$$w = -J\frac{k_\parallel}{K}e^{-k_\parallel d_1}, v = -J\frac{k_\parallel}{K}e^{-k_\parallel d_2}. \tag{31}$$

There are three interface states for this coupled SSH chain, as shown in Fig. S4(c). One of them is an exact zero mode corresponding to the zero energy, which comes from the analytical solution of eigenfunction $H\left|\phi_1\right\rangle = E_0\left|\phi_1\right\rangle = 0\left|\phi_1\right\rangle$ by assuming $\left|\phi_1\right\rangle = (x_1, x_2, ..., x_N)^T$. We have given the specific form of $\left|\phi_1\right\rangle$ in the main text. The rest two states correspond with the highest and lowest bands, respectively. This feature can be roughly explained by an extreme situation of Eq. (30) as shown in Fig. S4(d), where $w \gg v$ changes the Hamiltonian into

$$H \approx \sum_{s=1}^{(N+1-l_{\rm dw})/2} [w \left|l_{\rm dw}+2s-2\right\rangle_L \left\langle l_{\rm dw}+2s-1\right|_L + H.c.] \tag{32}$$
$$+ \sum_{s=1}^{l_{\rm dw}/2} [w \left|l_{\rm dw}-2s+2\right\rangle_L \left\langle l_{\rm dw}-2s+1\right|_L + H.c.].$$

In the above Hamiltonian, a trimer appears in the interface as

$$H_{\rm tri} = w\left(\left|l_{\rm dw}\right\rangle_L \left\langle l_{\rm dw}+1\right|_L + \left|l_{\rm dw}\right\rangle_L \left\langle l_{\rm dw}-1\right|_L\right) + H.c., \tag{33}$$

with all other $L$ branch states are connected by the strong coupling $w$ as a dimer

$$H_{\rm dim} = w\left|l\right\rangle_L \left\langle l+1\right|_L + H.c..$$

By applying the symmetric and anti-symmetric operations to the basis of the trimer and dimer, we have

$$H_{\rm tri} = \sqrt{2}w\left(\left|\phi_{\rm h}\right\rangle\left\langle\phi_{\rm h}\right| - \left|\phi_{\rm l}\right\rangle\left\langle\phi_{\rm l}\right|\right), \tag{34}$$
$$H_{\rm dim} = w\left(\left|\phi_+\right\rangle\left\langle\phi_+\right| - \left|\phi_-\right\rangle\left\langle\phi_-\right|\right).$$

with

$$|\phi_{\rm h}\rangle = \frac{1}{2}\left(|l_{\rm dw}+1\rangle_L + |l_{\rm dw}-1\rangle_L\right) + \frac{1}{\sqrt{2}}|l_{\rm dw}\rangle_L\,,$$
$$|\phi_{\rm l}\rangle = \frac{1}{2}\left(|l_{\rm dw}+1\rangle_L + |l_{\rm dw}-1\rangle_L\right) - \frac{1}{\sqrt{2}}|l_{\rm dw}\rangle_L\,,$$

and

$$|\phi_+\rangle = \frac{|l\rangle_L + |l+1\rangle_L}{\sqrt{2}}, |\phi_-\rangle = \frac{|l\rangle_L - |l+1\rangle_L}{\sqrt{2}}.$$

Apparently $|\phi_{\rm h}\rangle$ ($|\phi_{\rm l}\rangle$) is the interface state corresponding to the highest (lowest) band in this situation. Since $v/w = e^{-k_\parallel(d_2-d_1)} \approx 0.66$ for $k_\parallel = 0.1K$ in our consideration with $d_1 = 1\,{\rm nm}$ and $d_2 = 1.33\,{\rm nm}$, we have $|\phi_2\rangle \approx |\phi_{\rm h}\rangle$ and $|\phi_3\rangle \approx |\phi_{\rm l}\rangle$ as an approximation in the main text.

* wangyao@hku.hk


[1] Th. Forster, Energiewanderung und Fluoreszenz, Naturwissenschaften **33**, 166–175 (1946).

[2] Bing Shen Wang and Joseph L. Birman, Exciton dispersion in multiple quantum wells and superlattices: An additional contribution to the linewidth, Phys. Rev. B **43**, 12458 (1990).

[3] Judith F. Specht, Andreas Knorr, and Marten Richter, Two-dimensional spectroscopy: An approach to distinguish Förster and Dexter transfer processes in coupled nanostructures, Phys. Rev. B **91**, 155313 (2015).

[4] M. Selig, E. Malic, K. J. Ahn, N. Koch, and A. Knorr, Theory of optically induced Förster coupling in van der Waals coupled heterostructures, Phys. Rev. B **99**, 035420 (2019).

[5] H. Yu, G. Liu, P. Gong, X. Xu and W. Yao, Dirac cones and Dirac saddle points of bright excitons in monolayer transition metal dichalcogenides, Nat. Commun. **5**, 3876 (2014).

[6] H. Yu, X. Cui, X. Xu, and W. Yao, Valley excitons in two-dimensional semiconductors, Natl. Sci. Rev. **2**, 57–70 (2015).

[7] Diana Y. Qiu, Ting Cao, and Steven G. Louie, Nonanalyticity, Valley quantum phases, and lightlike exciton dispersion in monolayer transition metal dichalcogenides: theory and first-principles calculations, Phys. Rev. Lett. **115**, 176801 (2015).

[8] J. Z. Zhang and J. Z. Ma, Two-dimensional excitons in monolayer transition metal dichalcogenides from radial equation and variational calculations, J. Phys.: Condens. Matter **31**, 105702 (2019).

[9] I. S. Gradshteyn and I. M. Ryzhik, *Table of Integrals, Series, and Products* (Academic Press, 2014)

[10] D. Y. Qiu, F. H. da Jornada, and S. G. Louie, Optical spectrum of MoS2: many-body effects and diversity of exciton states, Phys. Rev. Lett. **111**, 216805 (2013).

[11] D. Xiao, G.-B. Liu, W. Feng, X. Xu, and W. Yao, Coupled spin and valley physics in monolayers of MoS2 and other group VI dichalcogenides, Phys. Rev. Lett. **108**, 196802 (2012).

[12] K. F. Mak, et al. Tightly bound trions in monolayer $MoS_2$. Nat. Mater. **12**, 207-211 (2013).

[13] J. S. Ross, et al. Electrical control of neutral and charged excitons in a monolayer semiconductor. Nat. Commun. **4**, 1474 (2013).

[14] N. S. Rytova, Screened potential of a point charge in a thin film, Proc. MSU, Phys. Astron. **3**, 30 (1967).

[15] L. V. Keldysh, Coulomb interaction in thin semiconductor and semimetal films, JETP Lett. **29**, 658 (1979).

[16] M. Danovich, D. A. Ruiz-Tijerina, R. J. Hunt, M. Szyniszewski, N. D. Drummond, and V. I. Fal'ko, Localized interlayer complexes in heterobilayer transition metal dichalcogenides, Phys. Rev. B. **97**, 195452 (2018).
